# Supplementary material for: Reducing Class-wise Confusion for Incremental Learning with Disentangled Manifolds
Source: arXiv:2503.17677 source file (2025-03-22)
Supplement: Supplementary file 1 [file X_suppl.tex]

\clearpage
\setcounter{page}{1}
\maketitlesupplementary

\section{Additional experiments}
\label{sec:cub}

We provide an additional comparison on the fine-grained dataset CUB-200 in Table \ref{tab:cub}. 
CUB-200 \citep{wah2011caltech} has 200 classes, with 11,788 images in total. We utilize ResNet18 (without pretraining) as the backbone, and set the memory buffer to 20 exemplars per class for all methods.
We evaluate the proposed method on B0 Inc20 and B100 Inc20. In a highly similar scenario, our method surpasses other methods. It outperforms PsHD (NeurIPS' 2024) \cite{fan2024persistence} up to 4.88\% on average accuracy, which benefits from the proposed architecture and the separation loss that jointly learn class-specific subspaces. 

\begin{table}[h]
\centering
\caption{Comparison on a fine-grained dataset CUB-200.}
\resizebox{0.48\textwidth}{!}{
\begin{tabular}{ccccccc}
\hline
\multirow{2}{*}{Methods} & \multicolumn{3}{c}{B0 Inc20} & \multicolumn{3}{c}{B100 Inc20} \\
 & \#P & Last & Avg & \#P & Last & Avg \\ \hline
BEEF & 111.70 & 49.07 & 56.15 & 67.02 & 63.73 & 66.11 \\
DSGD & 111.70 & \underline{58.10} & 59.75 & 67.02 & 67.35 & 68.80 \\
PsHD & 111.70 & 57.29 & \underline{59.77} & 67.02 & \underline{68.07} & \underline{68.97} \\
CREATE & 17.72 & \textbf{58.78} & \textbf{60.81} & 17.72 & \textbf{70.82} & \textbf{73.85} \\ \hline
\end{tabular}
}
\label{tab:cub}
\end{table}

\section{Additional ablation study}
\label{sec:discussion}

\subsection{Impact of exemplar size}

We conduct additional ablation experiments to evaluate the performance by varying the size of the exemplar set. In the CIFAR100 Base50 Inc10 setting, we record the performance with 20, 10, 5, and 3 exemplars stored for each class, as shown in \cref{supp-fecamandexemplar}(a). 
When the number of exemplars per class (EPC) is reduced from 20 to 10, the final accuracy decreases from 68.4$\%$ to 67.53$\%$, indicating stable performance. When the EPC is dramatically reduced to only 3 exemplars per class, the average accuracy drops from 75.52$\%$ to 73.55$\%$, resulting in a tolerable decrease of 1.97$\%$.

\begin{figure}[h]
\centering
\begin{subfigure}{0.49\linewidth}
\includegraphics[width=\linewidth]{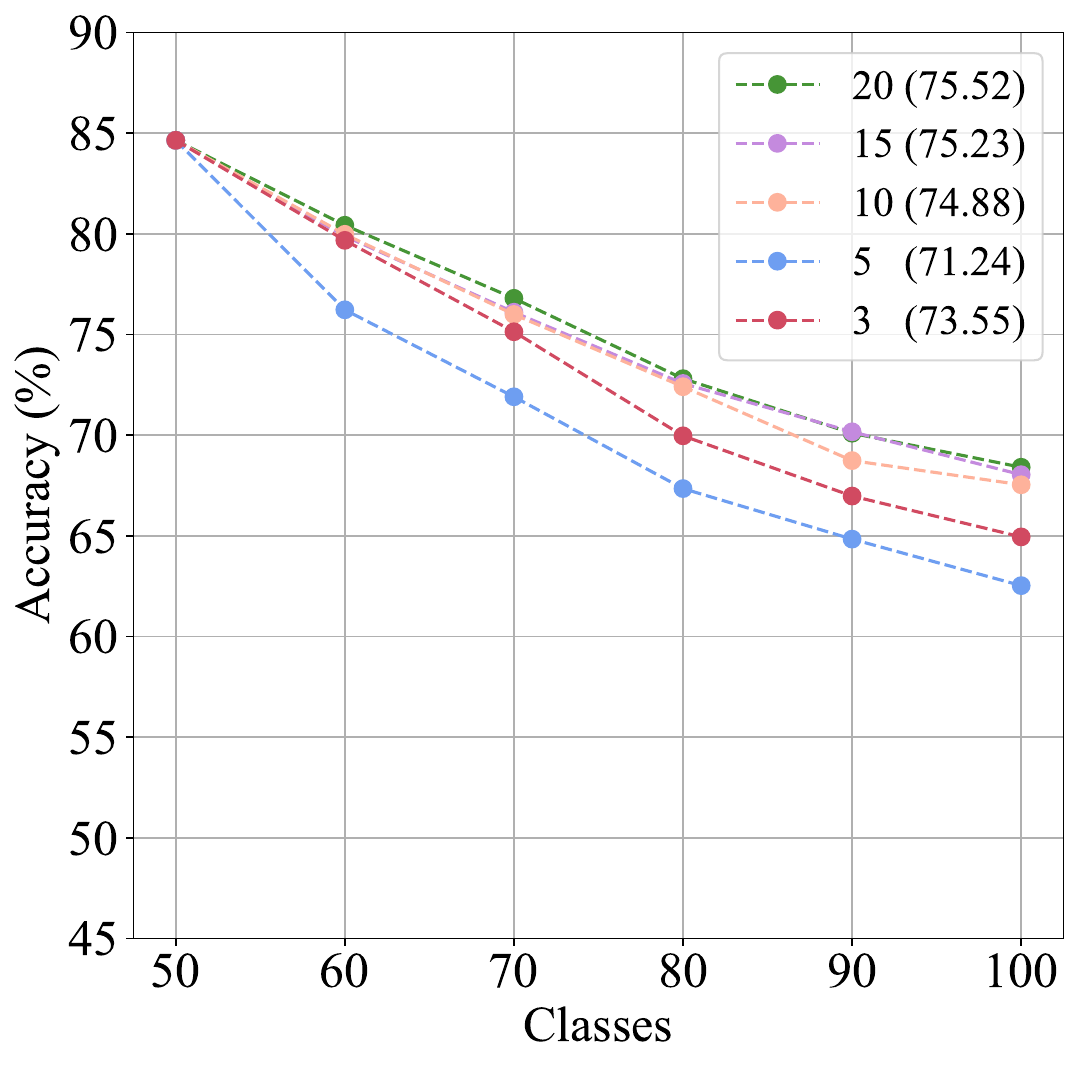}
\caption{exemplars per class}
\end{subfigure}
\begin{subfigure}{0.49\linewidth}
\includegraphics[width=\linewidth]{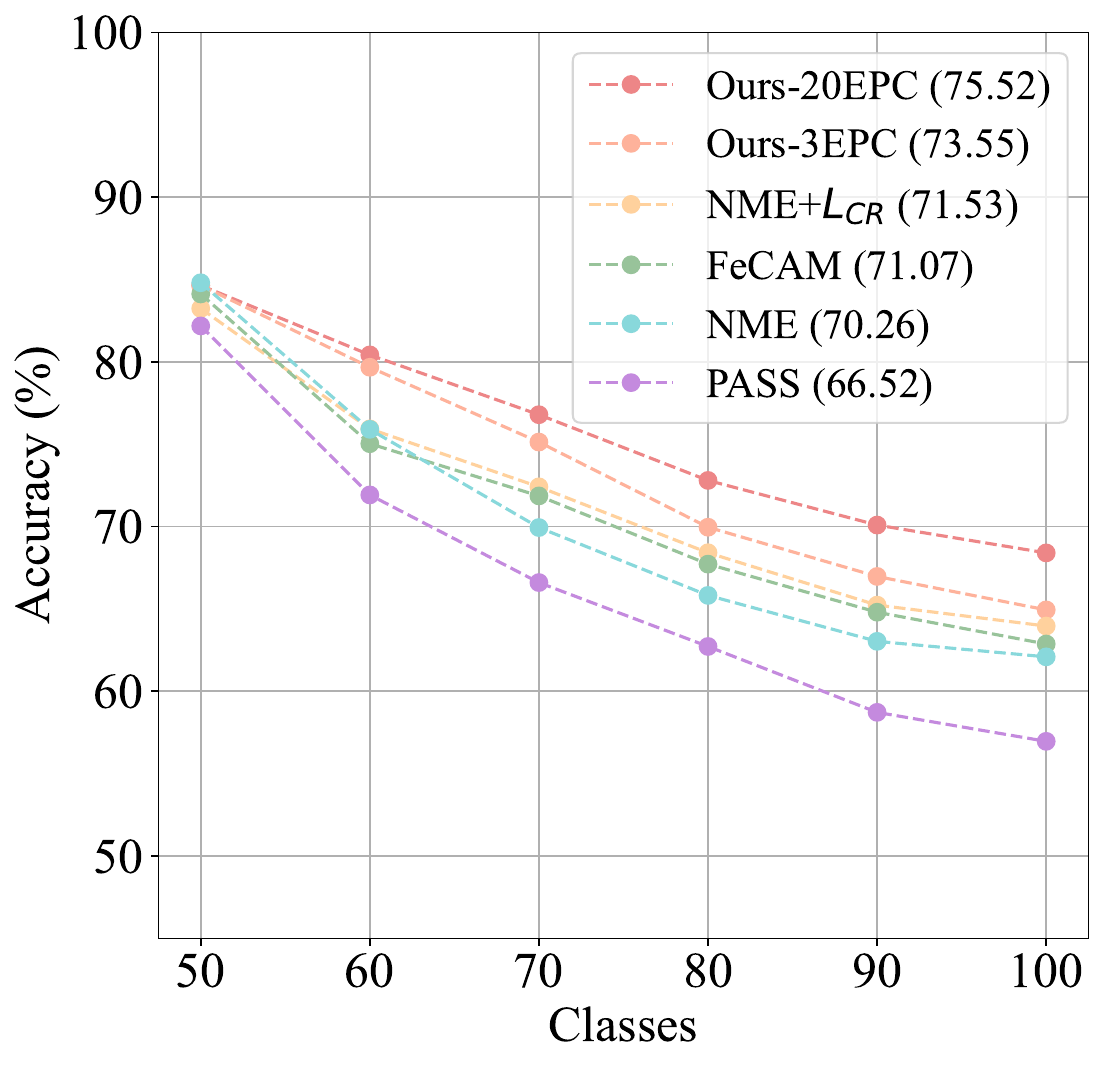}
\caption{baselines}
\end{subfigure}
\caption{Additional ablation study on different exemplar sizes and other baselines. The values in the parentheses in the legend represent the average accuracy. ``EPC'' is an abbreviation for ``exemplars per class''.}
\label{supp-fecamandexemplar}
\end{figure}

\subsection{Comparisons with exemplar-free methods}

Our proposed method is efficient and can achieve competitive performance compared with exemplar-free methods when adapted to lower storage or cost requirements.
FeCAM \cite{goswami2024fecam} is the SOTA of the exemplar-free methods, which proposes a feature covariance-aware metric based on prototypes for CIL. 
It stores a covariance matrix for each old class (106 MB in total), therefore, its memory cost is significantly higher than that of our proposed method CREATE when storing 3 exemplars per class (0.87 MB in total). 
PASS \citep{zhu2021prototype} freezes the backbone after the initial learning phase and stores one prototype for each class in the feature space. It requires 0.19 MB of memory but demands additional computation to implement self-supervised learning, augments rotation-based transformations for new samples, and adds Gaussian noise for prototypes. 
The experimental results are shown in \cref{supp-fecamandexemplar}(b). In the common exemplar-based setting, Ours-20EPC (20 exemplars per class) achieves a gain of 4.45$\%$ and 9.0$\%$ compared with FeCAM and PASS. Additionally, when converted to the corresponding memory overhead, Ours-3EPC (3 exemplars per class) shows a 2.48$\%$ improvement over FeCAM with a 99.18$\%$ reduction in storage cost and a 7.03$\%$ improvement over PASS with lower costs to learn new classes.

We also analyze the effectiveness of the $L_{CR}$ loss in the feature space without the reconstruction module, referred to as $NME+L_{CR}$. 
Experimental results indicate that using the $L_{CR}$ loss independently in feature space can also improve the performance of CIL by 1.27$\%$.

\subsection{Analysis of stability and plasticity}
To evaluate the performance improvements stemming from enhanced knowledge acquisition or reduced forgetting of the framework, we compare DER, BEEF, and our proposed method. The experiments are conducted using the CIFAR100 Base50 Inc50 set-up, where the number of old classes is the same as that of new classes. We evaluate the accuracy of old classes, new classes, and the overall accuracy. The experimental results are presented in \cref{supp-oldnew}. Our proposed method shows a 1.54$\%$ gap in learning new classes compared to previous methods, but it achieves approximately a 5$\%$ improvement in retaining old classes, significantly reducing the forgetting of old classes. Our method achieves a better balance between stability and plasticity.

\section{Pseudo code}
In \cref{algo}, we present the pseudo code for our proposed method CREATE.

\begin{algorithm}[h]
    \caption{CREATE}
    \begin{algorithmic}[1] % [1] 表示行号从1开始  
        \REQUIRE Dataset set $\mathcal{D} = \{\mathcal{D}_1, \mathcal{D}_2,..., \mathcal{D}_T\}$, seen class number in each phase $C=\{C_1, C_2, ...,C_T\}$, memory buffer $\mathcal{M}_t$, feature extractor $\phi_t$, classifier $\theta_t$, and auto-encoder module $AE_i$.
        \FOR{task t $\in$ [1, 2, ..., T]}
        
        \IF{t==1}
            \STATE Training set $\hat{\mathcal{D}_t} \gets \mathcal{D}_1$
            \STATE Create $AE_i$ for new class $i, i=\{0,...,C_1\}$
            \STATE Calculate cross-entropy loss $L_{CE}$ \COMMENT\cref{eq:lossce}
            \STATE Calculate confusion-reduce loss $L_{CR}$ \COMMENT\cref{eq:wcont}
            \STATE Train $\phi_t$ and $\theta_t$ by loss $L=L_{CE}+L_{CR}$
            
        \ELSE
            \STATE Training set $\hat{\mathcal{D}_t} \gets \mathcal{D}_t \bigcup \mathcal{M}_t$
            \STATE Freeze $\phi_{t-1}, \theta_{t-1}$, unfreeze $\phi_{t}$,
            \STATE Create $AE_i$ for new class $i, i=\{C_{t-1},...,C_t\}$
           
            \STATE Calculate cross-entropy loss $L_{CE}$ \COMMENT\cref{eq:lossce}
            \STATE Calculate knowledge distillation loss $L_{KD}$ according to the logits of ($\phi_{t-1},\theta_{t-1}$) \COMMENT{\cref{eq:losskd}}
            \STATE Calculate confusion-reduce loss $L_{CR}$ \COMMENT{\cref{eq:wcont}}
            \STATE Train $\phi_t$ and $\theta_t$ by loss $L=L_{CE}+L_{KD}+\lambda L_{CR}$ \COMMENT{\cref{eq:total}}
            
            \STATE Freeze $\phi_t$
            \STATE Training set $\mathcal{D}^{'}_t \gets$ sample a class-balanced subset from $M_{t-1}$ and $D_t$
            \STATE Fine-tune $\theta_t$ by \cref{eq:total}
        \ENDIF
        \STATE Old feature extractor $\phi_{t-1} \gets \phi_t$
        \STATE Old classifier $\theta_{t-1} \gets \theta_t$
        \STATE $\mathcal{M}_{t-1} \gets \mathcal{M}_{t}$
        \ENDFOR
    \end{algorithmic}  
\label{algo}
\end{algorithm}

\begin{figure}[t]
\centering
\includegraphics[width=\linewidth]{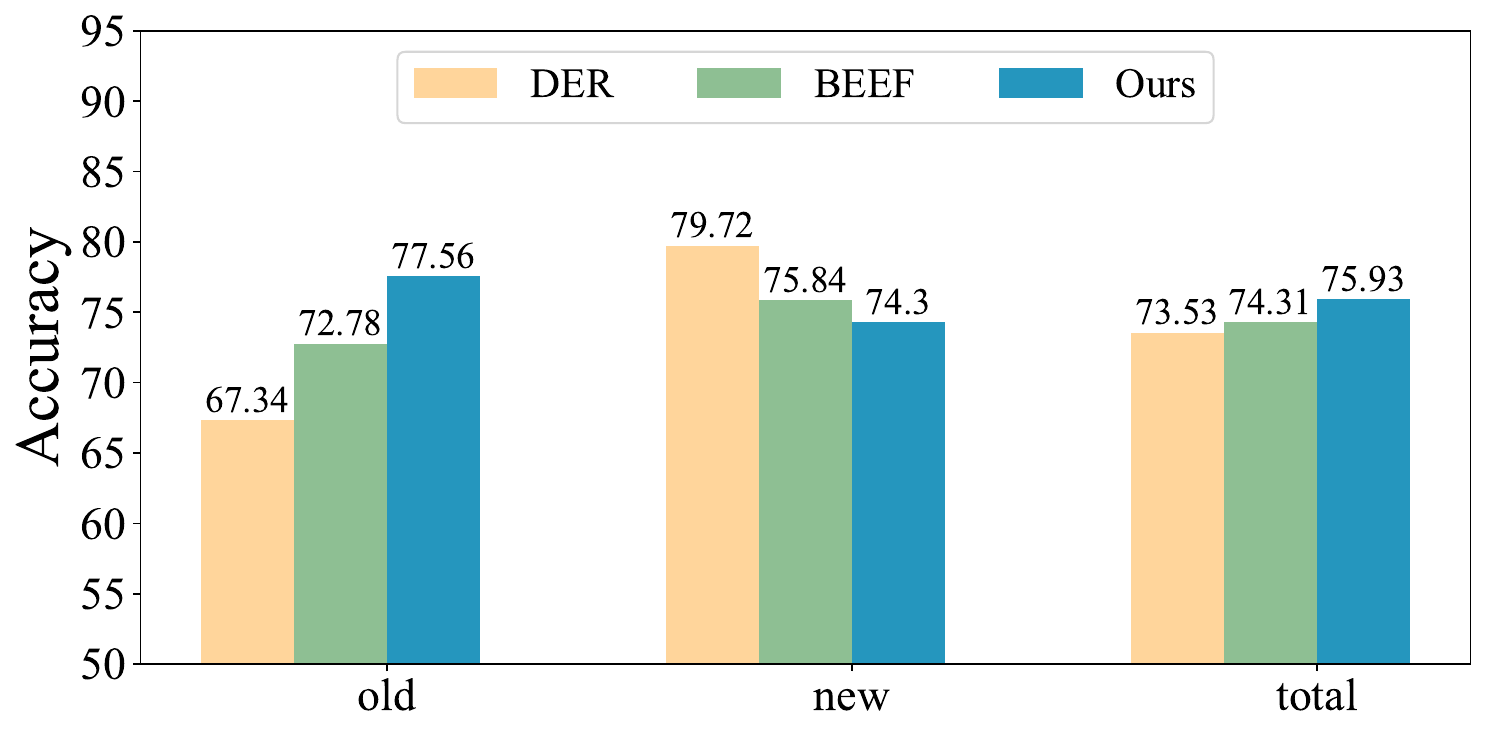}
\caption{The accuracy of old, new, and total classes on CIFAR100 Base50 Inc50. Our method achieves performance gains by mitigating forgetting more effectively than other methods.}
\label{supp-oldnew}
\end{figure}
