# Supplementary material for: Reducing Class-wise Confusion for Incremental Learning with Disentangled Manifolds
Source: arXiv:2503.17677 source file (2025-03-22)
Supplement: Supplementary file 2 [file 0_supp.tex]

\begin{abstract}

\begin{equation}
    e_i = \parallel \widetilde{h}_i - h \parallel .
\end{equation}

\begin{equation}
    p_i = \frac{\exp (-\alpha e_i)}{\sum_{j=1}^{C_t}{\exp (-\alpha e_j)}},
\label{eq:prob}
\end{equation}

\begin{equation}
    L_{CE}=-\sum_{i=1}^{C_t}  y_i \log p_i.
\label{eq:lossce}
\end{equation}

\begin{equation}
    L_{KD}= -\sum_{i=1}^{C_{t-1}} \frac{\exp(-\frac{\alpha \overline{e}_i}{T})}{\sum_{j=1}^{C_{t-1}}{\exp (- \frac{\alpha \overline{e}_j }{T})}} \log \frac{\exp(-\frac{\alpha e_i}{T}  )}{\sum_{j=1}^{C_{t-1}}{\exp (-\frac{\alpha e_j}{T})}},
\label{eq:losskd}
\end{equation}

\begin{equation}
    s_{i}=\frac{|{e_i}_{(2)} -
 {e_i}_{(1)}|}{{e_i}_{\max} - {e_i}_{(1)}},
\label{eq:score}
\end{equation}

\begin{equation}
   L_{CST} = \sum_{i=1}^{C_t} - \frac{1}{| P(i) |}\sum_{p\in P(i)} \log\frac{\exp(z_i^T \cdot z_{p_i} / \tau)}{\sum_{k\in S(i)} \exp(z_i^T \cdot z_{k_i} / \tau)},
\label{eq:cont}
\end{equation}

\begin{equation}
    w_{i}=1+e^{-\beta s_i}, w_i\in[1,2],
\label{eq:weight}
\end{equation}

\begin{equation}
    L_{CR}=\sum_{i=1}^{C_t} \frac{-1}{| P(i) |}\sum_{p\in P(i)} w_{i}\log\frac{\exp(z_i^T \cdot z_{p_i} / \tau)}{\sum_{k\in S(i)} \exp(z_i^T \cdot z_{k_i} / \tau)}.
\label{eq:wcont}
\end{equation}

\begin{equation}
    L = L_{CE}+L_{KD}+\lambda L_{CR},
\label{eq:total}
\end{equation}

\end{abstract}
